# Supplementary material for: Deep Optimized Priors for 3D Shape Modeling and Reconstruction
Source: arXiv:2012.07241 source file (2020-12-14)
Supplement: Supplementary file 1 [file dataset.tex]

\section{Dataset}\label{app:dataset}
In order to learn a better categorical prior, we further introduce a brand-new dataset, which are realistic and large-scale.
To create such a dataset, we add Bidirectional Reflectance Distribution Function (BRDF) materials to the shapes in ShapeNet \cite{}.
Firstly, we pre-process the selected shapes.
Next, the BRDF materials are applied to different parts of these shapes.
Finally, we set different light conditions and render images in different views.
The details are as following.

\noindent\textbf{3D Shape Collections --}
The 3D models to be textured come from a subset of ShapeNetCore V1, including 6 categories and over 25000 models.
Some of them do include material information either as Blinn-Phong parameters or as textures, but such materials are usually low quality and inadequate for photorealistic rendering.
During preprocessing, the initial 3D shapes vary in terms of geometric detail and quality, etc.
Moreover, most models lack UV mappings which are required for texturing.
To ensure the material can be applied to the shapes, we delete vertex doubles and enable smooth shading and use Blender's Smart UV projection algorithm for each material segment.

\noindent\textbf{Materials --}
The materials are represented as SVBRDFs with spatially varying diffuse, specular and roughness maps, which collected from \cite{Photoshape,Aittala,Vray-materials,merl}.
They also contain geometric information via normal and height maps.
This representation enables realistic reproduction of materials and seamless incorporation into any modern physically based renderer.

\noindent\textbf{Shape Rendering --}
We also have 30 lighting conditions from \cite{Photoshape} to simulate natural lighting conditions in all of our renderings.
We render each shape in different views, obtaining images and corresponding camera parameters.
